# Supplementary material for: How do infinite width bounded norm networks look in function space?
Source: arXiv:1902.05040 source file (2019-02-13)
Supplement: Supplementary file 1 [file smooth-appendix.tex]

\section{Proof of Theorem 1}

Consider a network $h_\Theta = f$ with $\lVert h_\Theta  \rVert = R(f)$.
\inote{
since the paper ends with my networks, 
it is best if you remind the readers you're dealing with
two layer networks
}

First, denote $\delta = \min_{x \neq x' \in B(f)} \frac{|x - x'|}2$, half the smallest gap between two breakpoints of $f$. For any $x_j \in B(f)$, we have:
	\begin{align}
	    \begin{split}
		f(x_j \pm \delta) &= 
		h_\Theta(x_j \pm \delta) = b^{(2)} + \sum_{i=1}^{k} w_i^{(2)} 
		\relu{w_i^{(1)} (x_j \pm \delta) + b_i^{(1)}} 
	    \end{split}
	\end{align}
	And, moreover, with 
	$\ind{z} = \mathbbm{1}\{z > 0\}$:
	\begin{equation}
	\begin{split}
		f'(x_j \pm \delta) &= h'_\Theta(x_j \pm \delta) = \sum_{i=1}^{k} w^{(1)}_i w_i^{(2)}
		\ind{w_i^{(1)} (x_j \pm \delta) + b_i^{(1)}}
	\label{eq-deriv_pm_delta2}
	\end{split}
	\end{equation}
	Note that $w_i^{(1)} (x_j \pm \delta) + b_i^{(1)} \neq 0$ for all units $i$: neither $x_j+\delta$ nor $x_j-\delta$ are breakpoints of $f$, 
	and since $h_\Theta = f$ there must be no change in the derivative of $h_\Theta$ at neither of the two points. 
	We can safely disregard multiple units activating at, 
	for example, $x_j+\delta$ since they would have to cancel each other's effect, 
	in which case the network would have suboptimal cost (removing such units would decrease its cost without affecting its output).
	
	From Equation \ref{eq-deriv_pm_delta2}, we can get:
	\begin{equation}
	\begin{split}
		f'(x_j + \delta) - f'(x_j - \delta) & = l_j - l_{j-1} 
		\\&= \sum_{i=1}^{k} w^{(1)}_i w_i^{(2)} \Big(\ind{w_i^{(1)} (x_j + \delta) + b_i^{(1)}} - \ind{w_i^{(1)} (x_j - \delta) + b_i^{(1)}}\Big)
	\label{eq-der_difference2}
	\end{split}
	\end{equation}
	Since units only activate or deactivate ($w_i^{(1)}x + b^{(1)}_i = 0$) at breakpoints of $f$, we have that 
	$\ind{w_i^{(1)} (x_j + \delta) + b_i^{(1)}} - \ind{w_i^{(1)} (x_j - \delta) + b_i^{(1)}} \neq 0$ if and only if $w_i^{(1)} x_j + b_i^{(1)} = 0$, 
	as $x_j$ is the only breakpoint in $[x_j - \delta, x_j + \delta]$. 
	Now, define:
	\begin{equation}
	\begin{split}
	    & \Gamma(x) = \{i : w_i^{(1)} x + b_i^{(1)} = 0\} \\
	    & \Gamma_+(x) = \{i \in \Gamma(x) : w^{(1)}_i > 0\}\\
	    & \Gamma_-(x) = \{i \in \Gamma(x) : w^{(1)}_i < 0\}
	\end{split}
	\end{equation}
    Then, we can rewrite Equation \ref{eq-der_difference2} as:
	\begin{equation}
	\begin{split}
		l_j - l_{j-1} &= \sum_{i \in \Gamma_+(x_j)} w^{(1)}_i w_i^{(2)} - \sum_{i \in \Gamma_-(x_j)} w^{(1)}_i w_i^{(2)} = \sum_{i \in \Gamma(x_j)} \pm w^{(1)}_i w_i^{(2)}
	\label{eq-slope_diff2}
	\end{split}
	\end{equation}
	Now, note that every unit $i \in [k]$ has a unique breakpoint in $B(f)$. Hence, we have $\bigcup_{x_j \in B(f)} \Gamma(x_j) = [k]$. By taking the absolute value and summing over all breakpoints:
	\begin{equation}
	\begin{split}
		\tv(f) = \sum_{j=1}^m |l_j - l_{j-1}| & \leq \sum_{j=1}^m \sum_{i \in \Gamma(x_j)} |w^{(1)}_i w_i^{(2)}| = \sum_{i=1}^k |w^{(1)}_i w_i^{(2)}| = \frac12 \lVert h_\Theta \rVert
	\end{split}
	\end{equation}
	where we used Lemma \ref{lemma-pal} in the last step and the definition of $\tv(\cdot)$.
	
	Now, note that we can assume w.l.o.g. that $\Gamma_+(x_j)$ and $\Gamma_-(x_j)$ only contain a single element (thus $|\sum_{i \in \Gamma_{\pm}(x_j)} w^{(1)}_i w_i^{(2)} | = \sum_{i \in \Gamma_{\pm}(x_j)} |w^{(1)}_i w_i^{(2)} |$), since we can always collapse all units into a single one as they have the same breakpoint $x_j$. Denote $\Lambda_+(x_j) = \sum_{i \in \Gamma_+(x_j)} w^{(1)}_i w_i^{(2)}$ and $\Lambda_-(x_j) = \sum_{i \in \Gamma_-(x_j)} w^{(1)}_i w_i^{(2)}$. We can write:
	\begin{equation}
	\begin{split}
		\Lambda_-(x_j) = \Lambda_+(x_j) + l_{j-1} - l_j
	\end{split}
	\label{eq-lambdapm}
	\end{equation}
	Using the previous equation and Lemma \ref{lemma-pal}, we can express the norm of the network as:
	\begin{equation}
	\begin{split}
		\lVert h_\Theta \rVert &= 2 \sum_{i=1}^k |w^{(1)}_i w^{(2)}_i| = 2 \sum_{j =1}^m \sum_{i \in \Gamma(x_j)} |w^{(1)}_i w^{(2)}_i| = 2 \sum_{j =1}^m \left( \sum_{i \in \Gamma_+(x_j)} |w^{(1)}_i w^{(2)}_i| + \sum_{i \in \Gamma_-(x_j)} |w^{(1)}_i w^{(2)}_i| \right) \\
		& = 2 \sum_{j = 1}^m \left( |\Lambda_+(x_j)| + |\Lambda_-(x_j)| \right) = 2 \sum_{j = 1}^m \left( |\Lambda_+(x_j)| + |\Lambda_+(x_j) + l_{j-1} - l_j| \right)
	\end{split}
	\end{equation}
	Now, take $x_p$ and $x_q$ two arbitrary points, where $l_p$ is the slope at $x_p$ (or at $x_p+\delta$, if $x_p \in B(f)$), and assume w.l.o.g. that $x_p < x_q$. Consider the following choices for $\Lambda_{\pm}(x_j)$, at breakpoints $B(f)$:
	\begin{equation}
	\begin{split}
	    \forall_{j \leq p} \quad &\Lambda_+(x_j) 
	    = 0 \quad \quad \Lambda_-(x_j) = l_{j-1} - l_j 
	    \\
		\forall_{j > p, j \neq q} \quad &\Lambda_+(x_j) = l_j - l_{j-1} \quad \quad \Lambda_-(x_j) = 0
		\\
		& \Lambda_+(x_q) = l_p + l_q - l_{q-1} \quad \quad \Lambda_-(x_q) = l_p
	\end{split}
	\end{equation}
	First, check that from Equation \ref{eq-lambdapm}, all changes in the slopes are satisfied. To see that this actually implements $f$, it suffices to note that $h'_\Theta(x_m + \delta) = \sum_{j=1}^m \Lambda_+(x_j) = l_p + l_q - l_{q-1} + \sum_{j=p+1: j \neq q}^m l_j - l_{j-1} = l_m$: since such parameters match all slope changes, and also match the slope $l_m$, then it must match all slopes. Now, check that, for such parameters:
	\begin{equation}
	\begin{split}
	    \lVert h_\Theta \rVert 
	    &=
	    2\left( |l_p + l_q - l_{q-1}| + |l_p| + 
	    \sum_{j = 1 : j \neq q}^m |l_j - l_{j-1}| \right) 
	    \\
	    &
	    = 2\left( |l_p + l_q - l_{q-1}| + |l_p| + \tv(f) - |l_q - l_{q-1}| \right)
	\end{split}
	\end{equation}
    In particular, we have two cases:
    \begin{itemize}
        \item $l_p + l_q - l_{q-1} \leq 0 \implies l_p \leq l_{q-1} - l_q$: In this case, we have $\lVert h_\Theta \rVert = 2 \cdot \tv(f)$
        
        \item $l_p + l_q - l_{q-1} > 0 \implies l_p > l_{q-1} - l_q$: In this case, we have $\lVert h_\Theta \rVert = 2 \Big( \tv(f) + 2(l_p - [l_{q-1} - l_q]_+) \Big)$
    \end{itemize}
    
    Moreover, if $x_q < x_p$:
    \begin{itemize}
        \item $l_p + l_{q-1} - l_q \leq 0$: In this case, we have $\lVert h_\Theta \rVert = 2 \cdot \tv(f)$
        
        \item $l_p + l_{q-1} - l_q > 0$: In this case, we have $\lVert h_\Theta \rVert = 2 \Big( \tv(f) + 2(l_p - [l_q - l_{q-1}]_+) \Big)$
    \end{itemize}

	Note that since this holds for arbitrary points $x_p$ and $x_q$, it also holds for points that minimize the cost. That is, for $\argmin l_i \leq \argmin_j l_j - l_{j-1}$:
	
	 \begin{itemize}
        \item If $\min_{i,j} l_i + l_j - l_{j-1} \leq 0$, then $R(f) = \lVert h_\Theta \rVert = 2 \cdot \tv(f)$
        
        \item If $\min_{i,j} l_i + l_j - l_{j-1} > 0$: then $R(f) = \lVert h_\Theta \rVert = 2 \Big( \tv(f) + 2(\min_{i,j} l_i - [l_{j-1} - l_j]_+) \Big)$
    \end{itemize}
    
    Moreover, for $\argmin l_i \geq \argmin_j l_j - l_{j-1}$:
	 \begin{itemize}
        \item If $\min_{i,j} l_i + l_{j-1} - l_j \leq 0$, then $R(f) = \lVert h_\Theta \rVert = 2 \cdot \tv(f)$
        
        \item If $\min_{i,j} l_i + l_{j-1} - l_j > 0$: then $R(f) = \lVert h_\Theta \rVert = 2 \Big( \tv(f) + 2(\min_{i,j} l_i - [l_j - l_{j-1}]_+) \Big)$
    \end{itemize}

\section{Bounds for $C^2$ Functions}

Unlike PWL functions which can be implemented by networks with at most countably infinite many units,
general $C^2$ functions require uncountably many neurons. 
For example, $f(x) = x^2$ has a change in derivative at any point $x \in \mathbb R$, meaning that to implement it, 
a new neuron would have to activate/deactivate at each point $x \in \mathbb R$ (or in any bounded interval).

To handle $C^2$ functions,
we first redefine networks with 1 hidden layer with $d$-dimensional inputs that can have uncountably many units:
\begin{equation}
    h_\alpha(x) = c + \int_{\mathbb S^{d-1} \times \mathbb R} \alpha(w,b) [\langle w, x \rangle + b]_+ \diff b
\end{equation}
For $1$-dimensional inputs, let us consider:
\begin{equation}
    h_\alpha(x) = c +  \sum_{w \in \{\pm 1\}} \int_{\mathbb R} \alpha(w,b) [w x + b]_+ \diff b
\label{eq-int_net}
\end{equation}
where $\alpha : \mathbb \{\pm 1\} \times \mathbb R \to \mathbb R$ maps the weight $w \in \{\pm 1\}$ and bias $b \in \mathbb R$ of a hidden unit to its outgoing weight $\alpha(w,b)$, and $c$ is the bias of the output unit. We only consider weights $w : |w| = 1$ since scaling $\alpha, b$ enables the same expressivity as $w \in \mathbb R$.

We also define the cost of an network of the form in Equation \ref{eq-int_net} as:
\begin{equation}
    \norm{ h_\alpha(x) }
    = 
    2 \sum_{w \in \{\pm 1\}} \int_{\mathbb R} |\alpha(w,b)| \diff b
\end{equation}
\inote{I don't get this definition...
it looks like $2\norm{\alpha}_1$.
Where does it come from?}
As present in {\color{red} citations on this}...

We now generalize our main results for functions $f \in C^2$:

\begin{theorem}[Implementation Cost of $C^2$ Functions with Stationary Points]

For any $C^2$ function $f: \mathbb R \to \mathbb R$, we have:
\begin{equation*}
	R(f) \geq 2 \cdot \tv(f)
\end{equation*}

Moreover, if $f$ has a stationary point, \eg $\exists_x, f'(x) = 0$, then:
\begin{equation*}
	R(f) = 2 \cdot \tv(f)
\end{equation*}

\end{theorem}

\begin{proof}
The proof follows from Lemma \ref{lemma-c2lb} and Lemma \ref{lemma-c2ub} below.
\end{proof}

\begin{lemma}[Implementation Lower Bound for $C^2$ Functions]
    \label{lemma-c2lb}
    For any $C^2$ function $f: \mathbb R \to \mathbb R$, we have:
    \begin{equation*}
    	R_2(f) \geq 2 \cdot \tv(f)
    \end{equation*}
\end{lemma}
\begin{proof}
	For any network 
	$h_{\alpha} 
	= 
	f$ 
	s.t. 
	$\norm{h_{\alpha}} = R(f)$, 
	and at any point $x$, 
	we have:
    \begin{align}
		f(x) &= h_\alpha(x) = c + \sum_{w \in \{\pm 1\}} \int_{\mathbb R} \alpha(w,b) [w x + b]_+ \diff b
		\\
		f'(x) &= h'_\alpha(x) = c + \sum_{w \in \{\pm 1\}} \int_{\mathbb R} \alpha(w,b) w \ind{w x + b} \diff b
	\end{align}
	and hence:
	\begin{equation}
		\frac{f'(x+\delta)  - f'(x)}\delta = \sum_{w \in \{\pm 1\}} \int_{\mathbb R} \alpha(w,b) w 
		\frac{ 
		\ind{w (x+\delta) + b} - \ind{w x + b} }{\delta} \diff b~.
	\end{equation}
	Taking $\delta \to 0$ we get
	\begin{equation}
		\lim_{\delta \to 0} \frac{f'(x+\delta)  - f'(x)}\delta = f''(x) = \lim_{\delta \to 0} \sum_{w \in \{\pm 1\}} \int_{\mathbb R} \alpha(w,b) w 
		\frac{
		    \ind{w (x+\delta) + b} - \ind{w x + b} 
		}{\delta} \diff b~.
	\end{equation}
	Now, let us generalize our definition of $\Gamma$ for the infinite case, and consider:
    \begin{align}
		\Gamma_+(x) &= \{(w,b) \in \{\pm1\} \times \mathbb R : wx + b = 0, w = 1 \} 
		\\
		\Gamma_-(x) & = \{(w,b) \in \{\pm1\} \times \mathbb R : wx + b = 0, w = -1 \}
	\end{align}
	Therefore,
	\begin{equation}
		f''(x) = \sum_{w \in \{\pm 1\}} \int_{\mathbb R} \alpha(w,b) w (\mathbbm 1 \{(w,b) \in \Gamma_+(x)\} \dirac{wx + b}) - \alpha(w,b) w (\mathbbm 1 \{(w,b) \in \Gamma_+(x)\} \dirac{wx + b}) \diff b
	\label{eq-diffdiracs}
	\end{equation}
	where $\dirac{z}$ allocates a point-mass to $z$.
    We can rewrite it as:
	\begin{equation}
		f''(x) = \int_{\mathbb R} \alpha(1,b) \dirac{x + b} + \alpha(-1,b) \dirac{-x + b} \diff b
	\end{equation}
	\begin{equation}
		f''(x) = \alpha(1,-x) + \alpha(-1,x)
	\end{equation}
    Now, using the triangle inequality, we get
	\begin{equation}
		\abs{f''(x)} = \abs{\alpha(1,-x) + \alpha(-1,x)} \leq \abs{\alpha(1,-x)} + \abs{\alpha(-1,x)}
	\end{equation}
	Now, we integrate over $\mathbb R$:
	\begin{equation}
		\tv(f) 
		= 
		\int_{\mathbb R} |f''(x)| \diff x 
		\leq
		\int_{\mathbb R} \abs{\alpha(1,-x)} + \abs{\alpha(-1,x)} \diff x 
		= 
		\sum_{w \in \{\pm 1\}} \int_{\mathbb R} \abs{\alpha(w,x)} \diff x
		=
		\frac{1}{2} \lVert h_\alpha \rVert = \frac12 R(f)
	\end{equation}
	
\end{proof}

\begin{lemma}[Implementation Upper Bound for $C^2$ Functions With Stationary Points]
For any $C^2$ function $f: \mathbb R \to \mathbb R$, such that $f$ has a stationary point, \eg $\exists_x, f'(x) = 0$, we have:
\begin{equation*}
	R_2(f) \leq 2 \cdot \tv(f)
\end{equation*}
\label{lemma-c2ub}
\end{lemma}

\begin{proof}
First, let $z$ denote an arbitrary stationary point of $f$: $f'(z) = 0$, and consider the following parameters $\alpha(w,b), c$:
\begin{equation}
\begin{split}
     &c = f(z) \\
    & \alpha(w,b) = \begin{cases}
f''(b), \text{ if } w=-1, b \in (-\infty, z]\\
f''(-b), \text{ if } w=+1, b \in (-\infty, -z]\\
0, \text{ otherwise} \\
\end{cases} 
\end{split}
\end{equation}
Then, we have:
	\begin{equation}
	\begin{split}
	    h_\alpha(x) &= f(z) + \sum_{w \in \{\pm 1\}} \int_{-\infty}^\infty a(w,b) [wx+b]_+ \diff b \\
	    & =
	    f(z) + \int_{-\infty}^z f''(b) [b-x]_+ \diff b + \int_{-\infty}^{-z} f''(-b) [x+b]_+ \diff b \\
	    & = 
	    f(z) + \int_{x}^z f''(b) (b-x) \diff b + \int_{z}^x f''(b) (x-b) \diff b \\
	    & = f(z) + \mathbbm 1 \{x \leq z\} \Big| b f'(b) - f(b) - xf'(b) \Big|_x^z + \mathbbm 1 \{x \geq z\} \Big|x'f(b) - bf'(b) + f'(b)\Big|_z^x \\
	    & = f(z) + \mathbbm 1 \{x \leq z\} \Big( f(x) - xf'(z) - f(z) + zf'(z) \Big) + \mathbbm 1 \{x \geq z\} \Big( f(x) - xf'(z) - f(z) + zf'(z) \Big) \\
	\end{split}
	\end{equation}
	and since $f'(z) = 0$, we get:
	\begin{equation}
	\begin{split}
	    h_\alpha(x) &= f(z) + \mathbbm 1 \{x \leq z\} \Big( f(x) - f(z) \Big) + \mathbbm 1 \{x \geq z\} \Big( f(x) - f(z) \Big) \\
	    & = f(z) + f(x) - f(z) = f(x)
	\end{split}
	\end{equation}
	Finally, check that:
	\begin{equation}
	\begin{split}
	    \lVert h_\alpha \rVert &= 2 \sum_{w \in \{\pm 1\}} \int_{\mathbb R} |\alpha(w,b)| \diff b = 2 \left(  \int_{-\infty}^z |f''(b)| \diff b + \int_{-\infty}^{-z} |f''(-b)| \diff b \right) \\
	    & = 2 \int_{-\infty}^\infty |f''(b)| \diff b = 2 \cdot \tv f
	\end{split}
	\end{equation}
	Hence proving the upper bound.
\end{proof}
